# Supplementary material for: A note on transience of generalized many-dimensional excited random walks
Source: arXiv:2211.05715 source file (2024-02-07)
Supplement: Supplementary file 1 [file AppendixB.tex]

\section{Proof of Proposition~\ref{prop41}}\label{proofpropR_n}\label{ap:A}

\input{proof_prop_Rn}
